# Supplementary material for: Strong Selection Significantly Increases Epistatic Interactions in the Long-Term Evolution of a Protein
Source: arXiv:1408.2761 ancillary file (2016-03-31)
Supplement: Supplementary file 1 [file Supporting-Gupta_Adami.pdf]

# Supporting Information

A. Gupta and C. Adami:
Strong Selection Significantly Increases Epistatic Interactions
in the Long-Term Evolution of a Protein

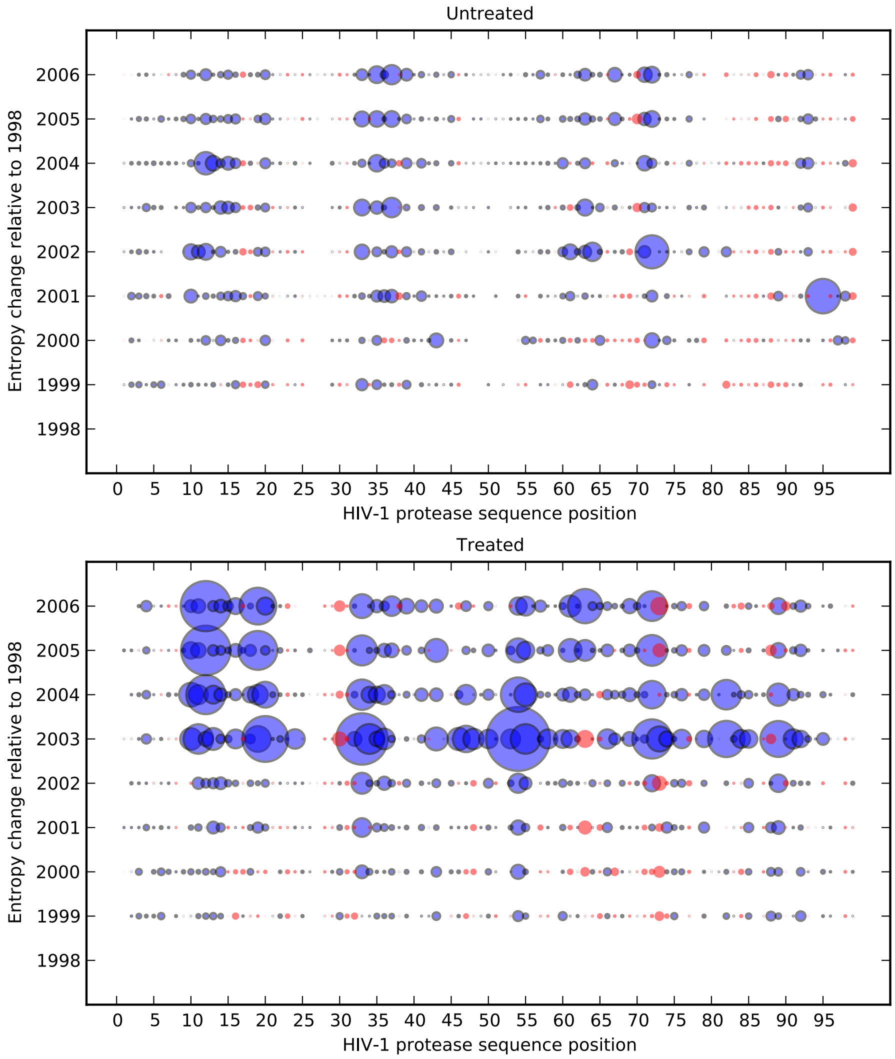


Figure S1: **Change in per-site entropies in HIV-1 protease over time.** Average entropy change (compared to 1998) at every position of the HIV-1 protease in the untreated (top panel) and treated (bottom panel) data sets. The size of the circles is proportional to the entropy change, and blue marks an increase while red implies a decrease in entropy at that site, compared to 1998 (the first year in our analysis). Site-specific variation mostly increased across the protein even in the absence of treatment, but decreased in some sites. In the treated data set, the entropy increased in most sites (in particular starting in 2003) while some sites became less entropic.

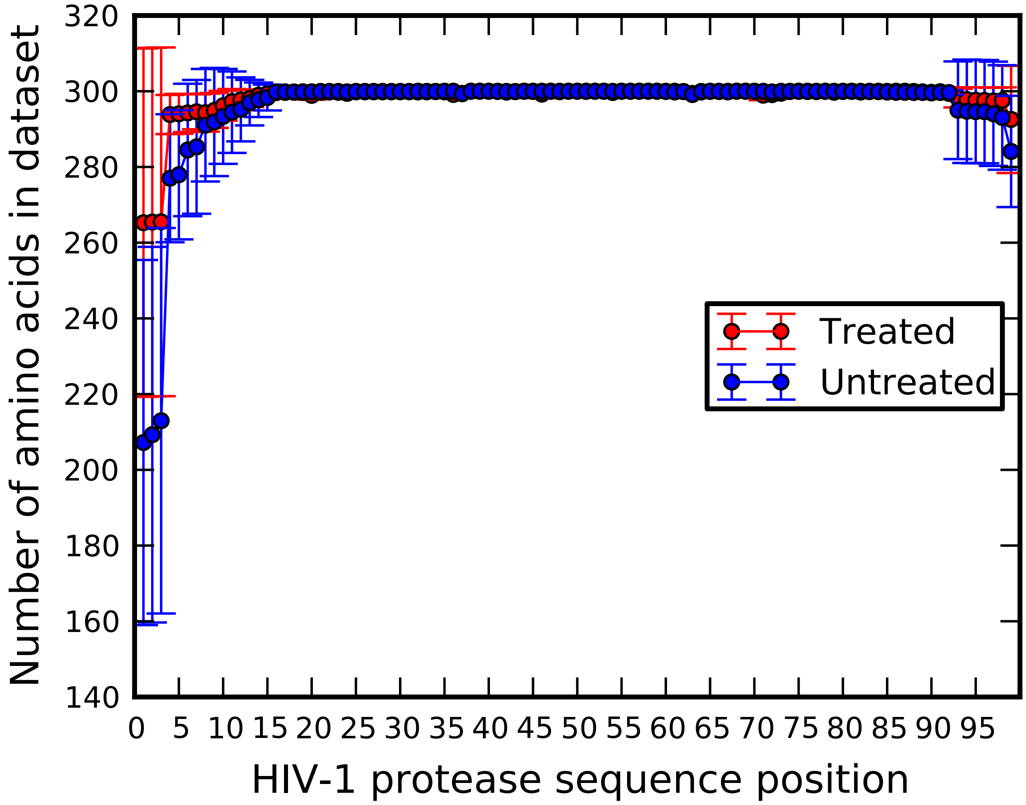


Figure S2: **Number of amino acids in each sampled set of 300 sequences for years 1998-2006.** Gaps at the beginning and ends of the protease sequence imply uneven sample size for positions $\geq$15 and $\leq$ 90, and thus the ends were truncated for calculation of per-site entropies and pairwise mutual information. Filled circles represent average number of residues in the sampled sets at each protease position and error bars represent unit SD.

**Supporting Table S1. Protease Inhibitors (PIs) and the years they were approved by FDA.** New drugs with higher genetic barriers to resistance are continually developed to provide treatment options to patients showing resistance to earlier drugs.

| Drug (PI) | Year | Comment |
|---|---|---|
| Saquinavir | 1996 | 1st-line PI, given with Ritonavir |
| Indinavir | 1996 | 1st-line PI. Metabolized quickly, requiring multiple doses per day to avoid drug resistance |
| Ritonavir | 1996 | Initially used as a 1st-line PI, now used in combination with other PIs due to its ability to metabolize the enzyme that metabolizes other PIs |
| Nelfinavir | 1997 | 1st-line PI |
| Amprenavir | 1999 | Discontinued in 2004, prodrug version still available (Fosamprenavir) |
| Lopinavir | 2000 | 2nd-line PI, given with Ritonavir in patients with some drug resistance |
| Atazanavir | 2003 | 2nd-line PI, given with Ritonavir in patients with some drug resistance |
| Fosamprenavir | 2003 | Slow-release version of Amprenavir |
| Tipranavir | 2005 | 2nd-line PI, given with Ritonavir in patients with some drug resistance |
| Darunavir | 2006 | 2nd-line PI, given with Ritonavir in patients with some drug resistance |

## Supporting Text S1: Phylogenetic structure of protease sequence data

We obtained protease sequences from the HIV Stanford Database [1, 2] that compiles data from several different sources. Although it has been shown that due to the high mutation rate of HIV-1, most amino acid covariation results from selection pressure and not linkage disequilibrium [3], we constructed the phylogenetic trees to rule out any confounding phylogenetic effects [4]. Only trees for even years are shown, although data from all years show similar star-like phylogeny.

Since we resampled 300 sequences from sequences available for each year and environment (treated and untreated), we show neighbor joining trees for each of these resampled datasets. The figures were made using the phylogeny inference package Phylip, where we used program *protdist* to compute distances between all pairs of sequences for constructing the neighbor joining trees [5]. All the trees show star-phylogeny, ruling out subdivisions in the data due to phylogenetic effects. The trees made with 100 bootstraps also showed star-like phylogenies (data not shown).

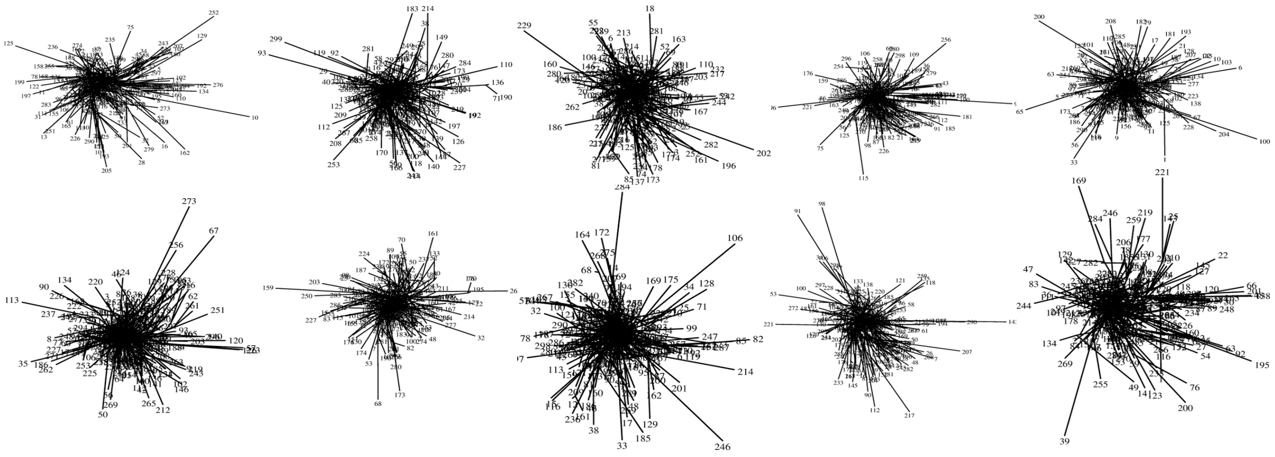

Phylogenies of subsampled datasets from year 1998 (untreated sequences)

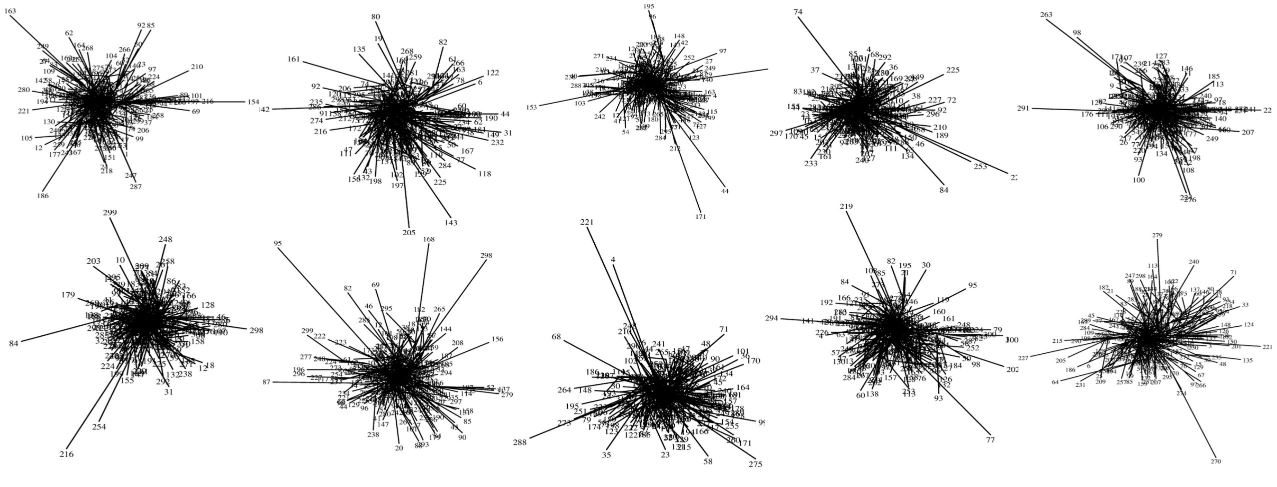

Phylogenies of subsampled datasets from year 2000 (untreated sequences)

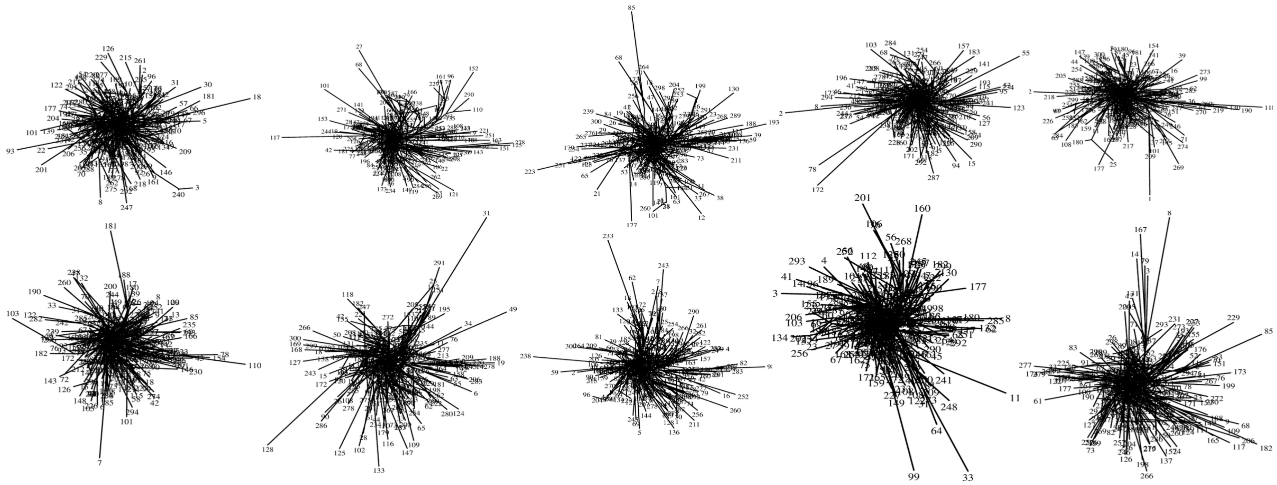

Phylogenies of subsampled datasets from year 2002 (untreated sequences)

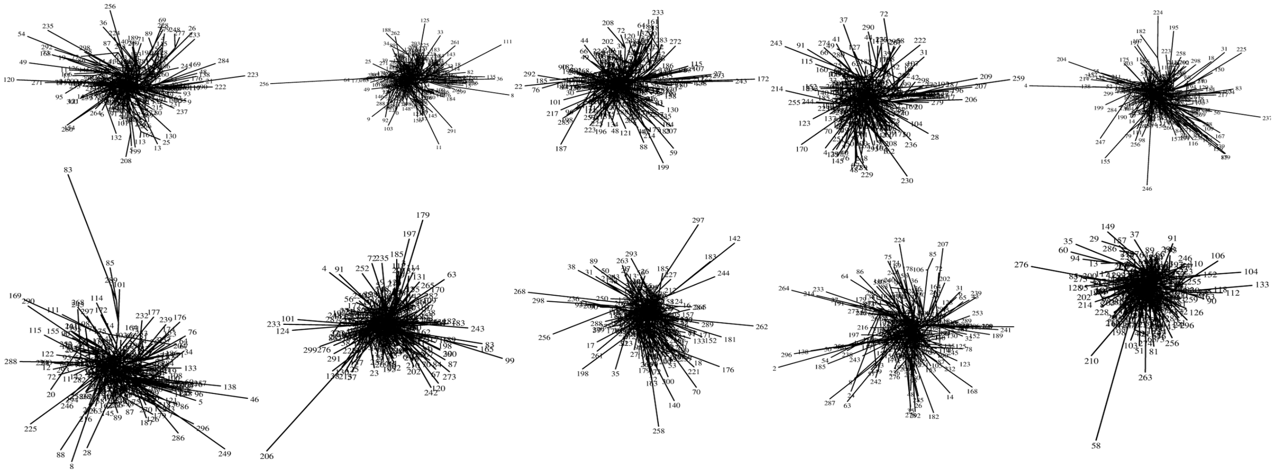

Phylogenies of subsampled datasets from year 2004 (untreated sequences)

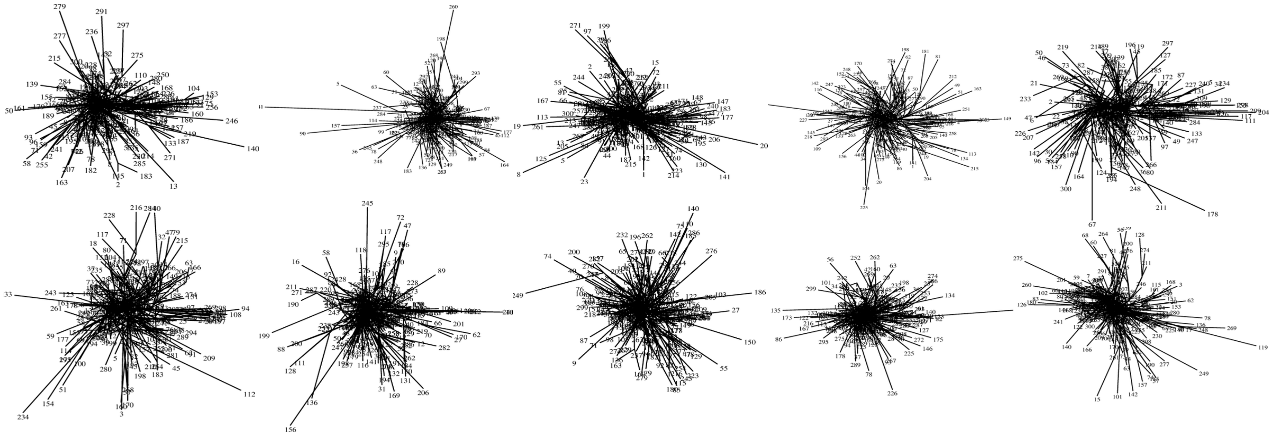

Phylogenies of subsampled datasets from year 2006 (untreated sequences)

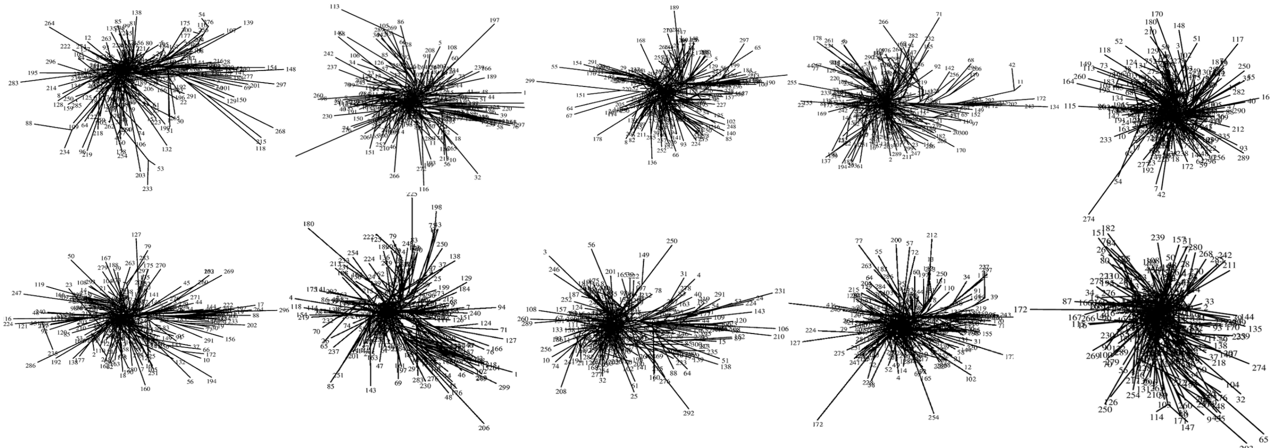

Phylogenies of subsampled datasets from year 1998 (treated sequences)

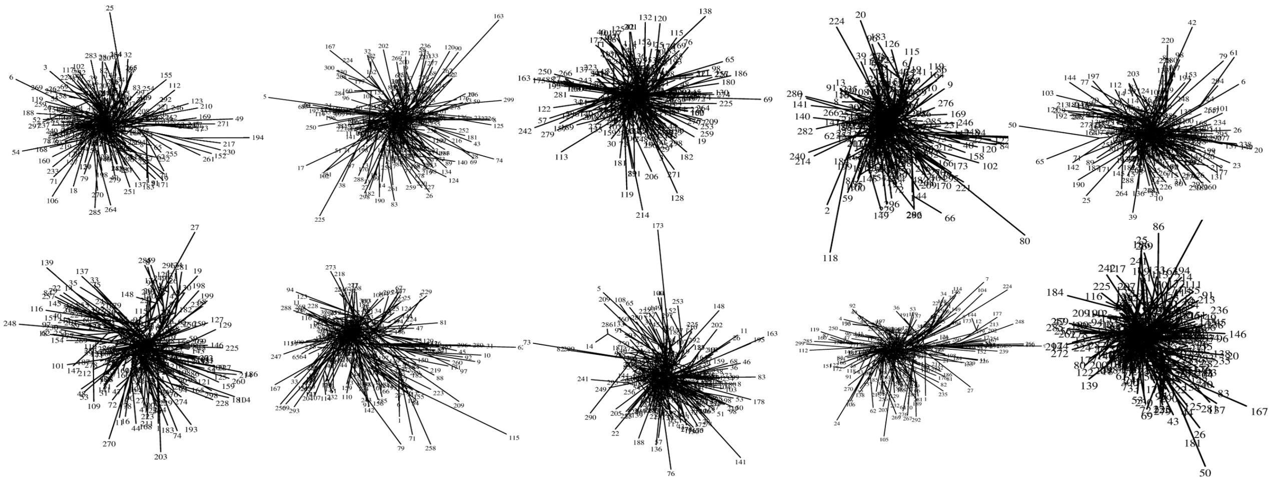

Phylogenies of subsampled datasets from year 2000 (treated sequences)

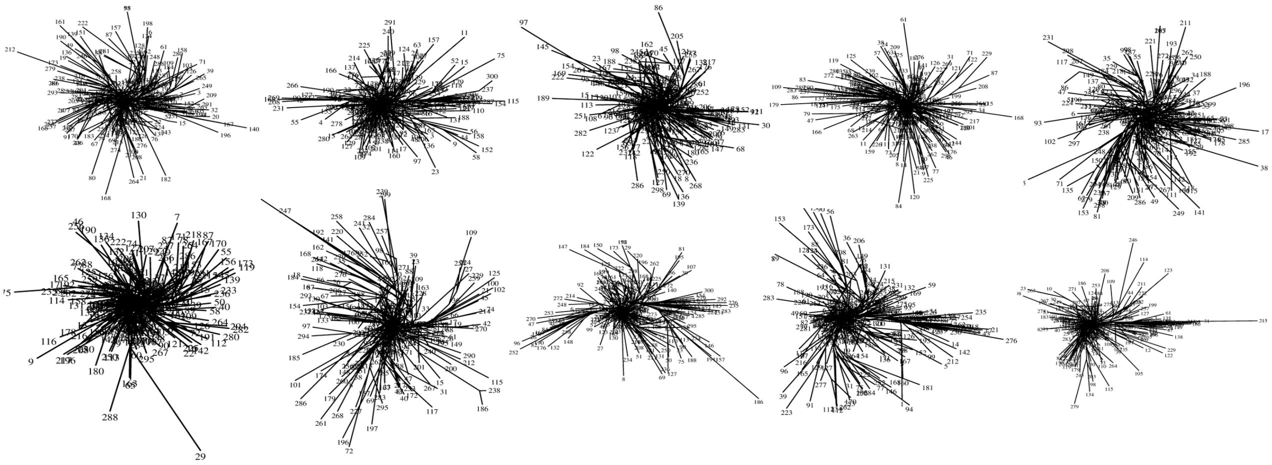

Phylogenies of subsampled datasets from year 2002 (treated sequences)

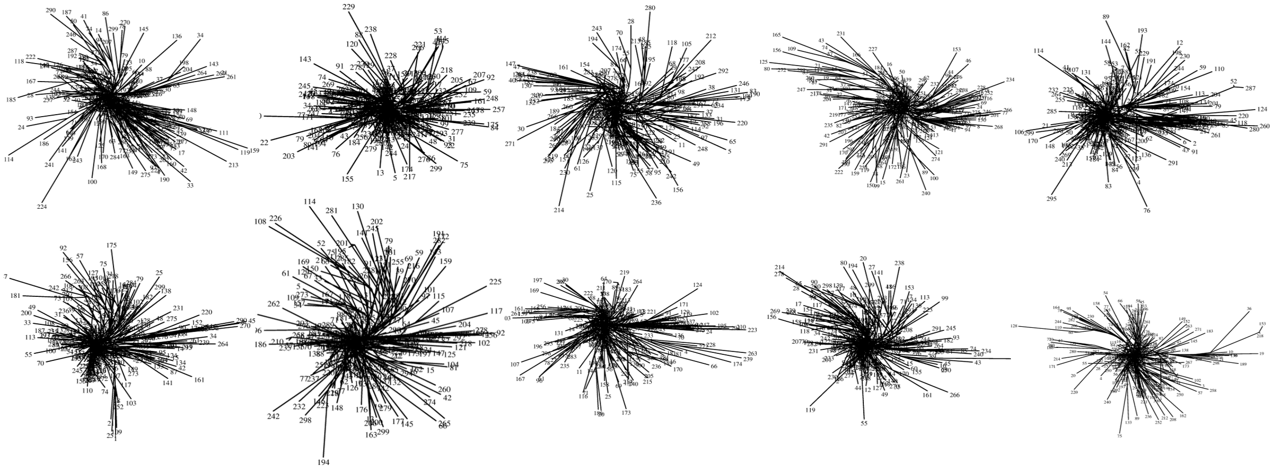

Phylogenies of subsampled datasets from year 2004 (treated sequences)

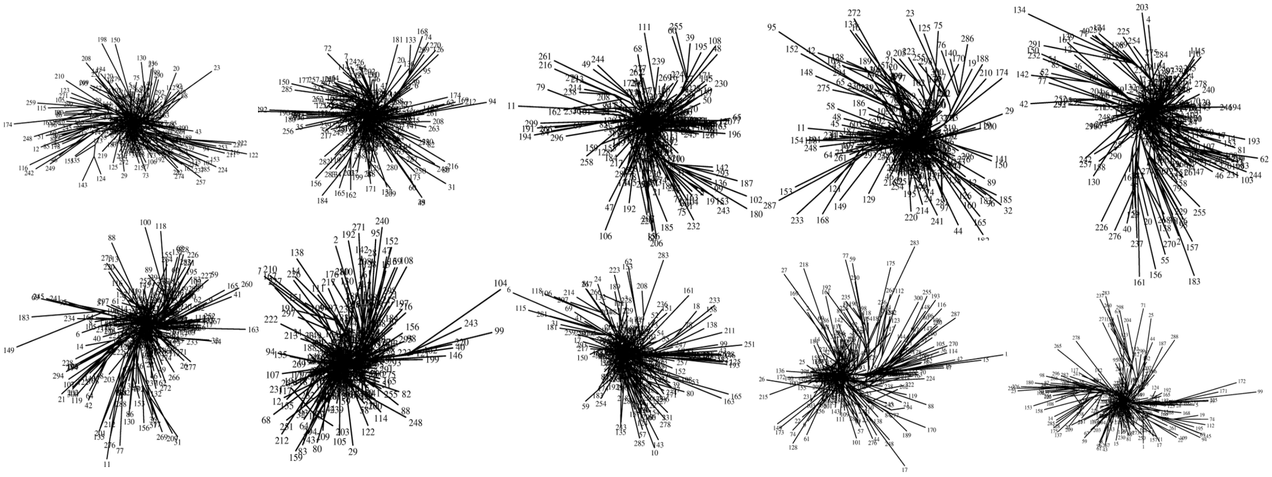

Phylogenies of subsampled datasets from year 2006 (treated sequences)

## References

[1] Rhee SY, Gonzales MJ, Kantor R, Betts BJ, Ravela J, Shafer RW. Human immunodeficiency virus reverse transcriptase and protease sequence database. Nucleic Acids Res. 2003;31:298–303.

[2] Shafer RW. Rationale and uses of a public HIV drug-resistance database. J Infect Dis. 2006;194 Suppl 1:S51–8.

[3] Wang Q, Lee C. Distinguishing functional amino acid covariation from background linkage disequilibrium in HIV protease and reverse transcriptase. PLoS One. 2007;2:e814.

[4] Lunzer M, Golding GB, Dean AM. Pervasive cryptic epistasis in molecular evolution. PLoS Genet. 2010;6:e1001162.

[5] Felsenstein J. PHYLIP- Phylogeny Inference Package. Cladistics. 1989;5:164–166.

## Supporting Text S2: Sequence Logos for HIV-1 Protease treated and untreated sequences.

Sequence logos from our treated and untreated HIV-1 protease data from all years are shown below (logos generated using Weblogo [1]). The residues are colored according to their chemical properties: polar residues as green; neutral residues as purple; basic residues as blue; acidic residues as red; and hydrophobic residues as black.

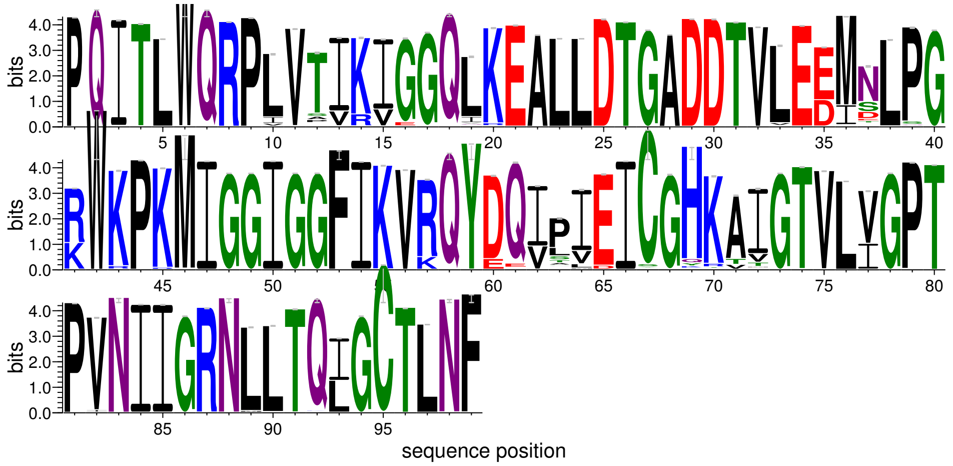

Sequence logo for the untreated protease sequences from all years.

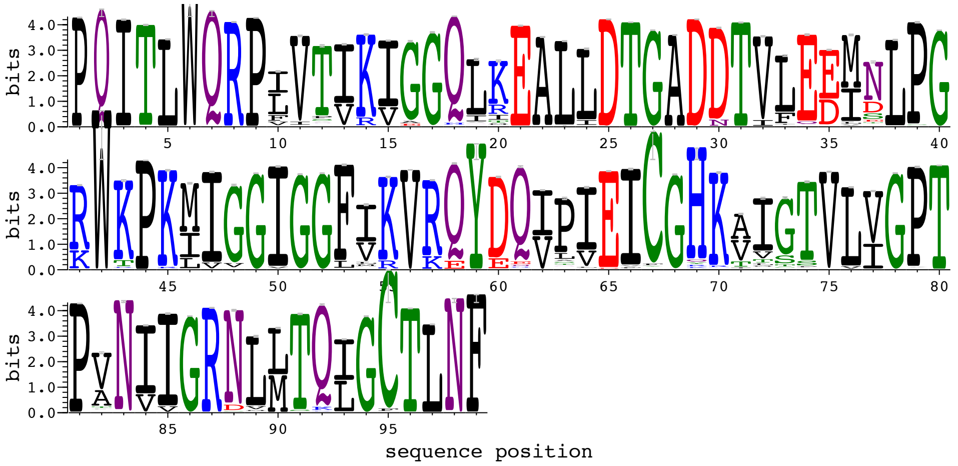

Sequence logo for the treated protease sequences from all years.

## References

[1] Crooks GE, Hon G, Chandonia JM, Brenner SE. WebLogo: a sequence logo generator. Genome Res. 2004;14:1188–1190.

## Supporting Text S3: Changes in physico-chemical properties at protease positions mirror per-site entropy changes

Our analysis of residue properties show that the increase in entropy is often associated with changes in residue charge or size at that position (Figure 2 main text). The "isoelectric point" (pI) is the pH at which there is no charge on the residue: positively charged residues have a higher pI (Arg R: 10.76, Lys K: 9.74) and negatively charged residues have a low pI (Asp acid D: 2.77, Glu acid E: 3.22, see Table below for pI and residue-weight of all residues). A negative pI difference implies that residues with a higher isoelectric point (more positively charged, thus more basic) are replaced by acidic and negatively charged residues upon treatment (Figure 2, main text, middle panel). Positive pI difference means that position is becoming more basic upon treatment. For position 30, although the entropy increase is not as significant as that at other loci, the loss of negative charge at the position (mutation from aspartic acid to asparagine, a major drug-resistance mutation) is substantial (Figure 2, main text, middle panel). Position 20, on the other hand, shows a decrease in pI following treatment, suggesting that the position has become more acidic.

Several protease positions also show a marked shift in residue-weight at positions post-treatment. The residue-weight difference at a position is positive when heavier residues occupy that position after treatment, as is the case for positions 71 (emergence of valine in place of alanine: A71V), 73 (serine is preferred to glycine in some treated sequences: G73S), and 90 (methionine replaces leucine in 50% of treated sequences, L90M; Figure 2, bottom panel in main text). These heavier residues seen in treated protease sequences are also larger in size than the residues in untreated sequences, and thus could create potential steric clashes unless compensatory mutations occur elsewhere. We also observe negative residue-weight differences at positions 36, 46, 54, and 83, suggesting that smaller residues are now occupying these positions to either avoid steric clashes due to other changes in the protein (accessory mutations), or to change the protein-drug interaction (resistance causing mutations).

**Physico-chemical properties of residues**

| Residue | Isoelectric point (pI) | Residue weight* |
|---|---|---|
| A | 6.0 | 71.08 |
| C | 5.07 | 103.15 |
| E | 3.22 | 129.12 |
| D | 2.77 | 115.09 |
| G | 5.97 | 57.05 |
| F | 5.48 | 147.18 |
| I | 6.02 | 113.16 |
| H | 7.59 | 137.14 |
| K | 9.74 | 128.18 |
| M | 5.74 | 131.2 |
| L | 5.98 | 113.16 |
| N | 5.41 | 114.11 |
| Q | 5.65 | 128.13 |
| P | 6.3 | 97.12 |
| S | 5.68 | 87.08 |
| R | 10.76 | 156.19 |
| T | 5.6 | 101.11 |
| W | 5.89 | 186.22 |
| V | 5.96 | 99.13 |
| Y | 5.66 | 163.18 |

*Residue weight = Molecular weight of amino acid - $H_2O$

Reference: D.R.Lide, Handbook of Chemistry and Physics, 72nd Edition, CRC Press, Boca Raton, FL, 1991.

http://www.sigmaaldrich.com/life-science/metabolomics/learning-center/amino-acid-reference-chart.html

## Supporting Text S4: Changes in epistatic interactions in a longitudinal study

The information content trends we highlighted in Figure 3 of the main text are obtained from pooled data taken from many different subjects. To test whether the trends also hold within patients, we analyzed the changes in information content and epistasis from patients enrolled in a longitudinal study. These data (HIV Stanford database, see Methods, protease sequences derived from the same patient at two time-points: first and second isolate) further support the observation that treatment decreases $I_1$ but increases the sum of pairwise mutual information, *i.e.*, treatment increases per-site variability as well as the extent of epistatic interactions in the protein. For patients that went from 'untreated' to 'treated' state, as well as patients that continued treatment, $I_1$ showed a slight decrease in the latter isolate.

Stopping treatment shows a slight increase in $I_1$, suggesting that entropy (amino acid variation) decreases when the selection pressure of drugs is removed, however, this observation is based on a small sample size (153 sequences in 'treated to untreated' category). The sum of pairwise mutual information also increases when treatment is initiated or continued, suggesting that information is redistributed towards interactions upon treatment. We note that while the longitudinal data agrees with the temporal trends for $I_1$ and $I_2$, it does not add statistical power to those conclusions due to small sample sizes.

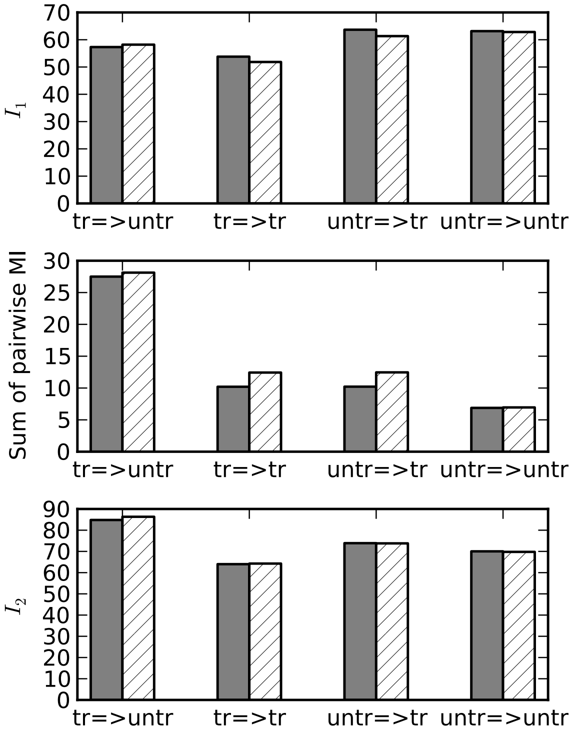


**Information measures from longitudinal data.** The categories are treated to untreated (tr=>untr), treated to treated (tr=>tr), untreated to treated (untr=>tr), and untreated to untreated (untr=>untr). Grey and hatched bars represent the first and second time-point, respectively. $I_1$ decreases as entropy increases due to treatment (top panel), while sum of pairwise mutual information increases due to treatment (middle panel). The net information content of the protein, as approximated by $I_2$, does not show any change in the two isolates collected from the same patient.

## Supporting Text S5: Information between epistatic pairs in protease of treated and untreated subjects, for spatially close and distant epistatic residue pairs

We analyze the redistribution of information between epistatic pairs over time, separating out spatially close from distant residues. We show the cumulative distribution of information as a function of $\log_{10}$ of information, separately for close residues (those that are thought to be in contact) and those that are distant from each other. As criterion for "closeness" we use a cutoff of $8\mathring{A}$ distance between residues in the 3D structure, as is usual in the literature for contact prediction [1, 2, 3]. We separately analyze the interacting pairs within the molecule for early, medium, and late time points as well as for treated and untreated groups (using a larger cutoff such as $10\mathring{A}$ does not change the trend).

Inter-residue distances were determined using Bio.PDB, a biopython module for analysis of crystallographic structures [4]. Since the protease is a dimer but the sequence data is that of a single chain, we assume that both chains are identical and compute distances between residues from protease chain A in PDB structure 1F7A [5, 6].

For the sequences from 1998 (left panel), there was little difference in treated and untreated subjects in the distribution of information for close pairs (contacts), but significant difference in the information for distant pairs: the untreated subjects were storing more information in distant pairs than the treated subjects. This trend is reversed already in the year 2002 (middle panel), and more significantly in 2006 (right panel). For those years, molecules under treatment stored more information in pairs than those not under selection, but the significant difference between the trend in close vs. distant residues has all but disappeared by 2006, meaning that the interactions between residues over long-distances (see for example in Fig. 5 of the main text, which have also been observed in other proteins [3]) have disappeared both in the treated as well as the untreated subjects. It is not clear if the effect is solely due to the long-term evolution of the protease or due to complex treatment histories of patients on antiviral therapies.

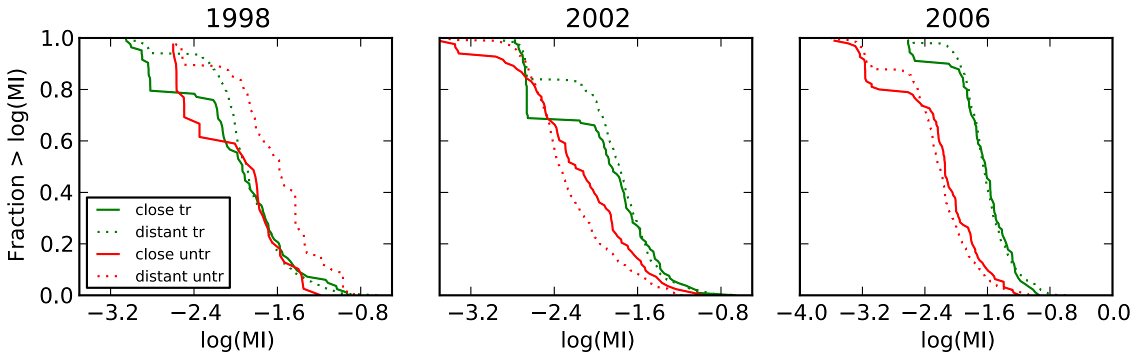


**Cumulative distribution of epistatic information for the years 1998, 2002, and 2006.** Information in pairs that are in-contact (residue distance $< 8\mathring{A}$), labeled 'close', solid lines), and distant residues (dashed lines, residue distance $\geq 8\mathring{A}$) as a function of the $\log_{10}$ of the mutual information of the pairs. Cumulative distribution for treated subjects in green, for untreated subjects in red. Only pairs with significant mutual information are included.

## References


[1] Fodor AA, Aldrich RW. Influence of conservation on calculations of amino acid covariance in multiple sequence alignments. Proteins. 2004; 56:211–21.

[2] Shackelford G, Karplus K. Contact prediction using mutual information and neural nets. Proteins. 2007; 69 Suppl 8:159–64.

[3] Burger L, van Nimwegen E. Disentangling direct from indirect co-evolution of residues in protein alignments. PLoS Comput Biol. 2010; 6:e1000633.

[4] Cock PJA, Antao T, Chang JT, Chapman BA, Cox CJ, Dalke A, et al. Biopython: freely available Python tools for computational molecular biology and bioinformatics. Bioinformatics. 2009; 25:1422–3.

[5] Bernstein FC, Koetzle TF, Williams GJ, Meyer EF Jr, Brice MD, Rodgers JR, et al. The Protein Data Bank: a computer-based archival file for macromolecular structures. Arch Biochem Biophys. 1978; 185:584–91.

[6] Prabu-Jeyabalan M, Nalivaika E, Schiffer CA. How does a symmetric dimer recognize an asymmetric substrate? A substrate complex of HIV-1 protease. J Mol Biol. 2000; 301:1207–20.

# Supporting Text S6: Correction for sample-size bias in entropy and mutual information estimates

It is well-known that entropy and information estimations from frequencies (maximum-likelihood estimators) are unreliable when sample sizes are small, due to under-sampled probability distributions [1]. Because total information estimation sums over $n(n-1)/2$ residue pairs, it is important to correctly estimate entropies so as not to accumulate finite sample-size errors. We tested several estimators for entropy and, in particular, information calculations:

**Maximum likelihood (ML) estimator**: empirical values of entropy calculated from observed frequencies.

**Miller Madow (MM) estimator**: bias-corrected empirical entropy estimator [2].

**Jeffreys estimator**: Bayesian estimates of the bin frequencies using the Dirichlet-multinomial pseudocount model (pseudocount = 1/2) [3].

**Laplace's prior**: Bayesian estimates of the bin frequencies using the Dirichlet-multinomial pseudocount model (pseudocount = 1).

**SG estimator**: Bayesian estimates of the bin frequencies using the Dirichlet-multinomial pseudocount model, pseudocount = 1/20 (since 20 amino acids) [4].

**Minimax estimator**: Bayesian estimates of the bin frequencies using the Dirichlet-multinomial pseudocount model, pseudocount = $\sqrt{n}/20$ (n = number of sequences, 20 because of 20 possible residues at each position).

**Chao Shen (CS) estimator**: Proposed by Chao and Shen in 2003 [5].

**Shrink estimator**: Proposed by Hausser and Strimmer in 2009 [6].

**NSB estimator**: Proposed by Nemenman, Shafee, and Bialek [7].

To compare the performance of these estimators as sample size is increasing, we computed entropies at positions 54 and 82 of HIV-1 protease (a pair that is known to show substantial correlation [8]) for the 2003 treated data for gradually increasing sample sizes (total number of sequences in this data = 3319). As seen in the figure below, entropy and information estimates improve as sample size increases. Based on this analysis, we chose the NSB entropy estimator for our subsampled datasets of size 300 each.

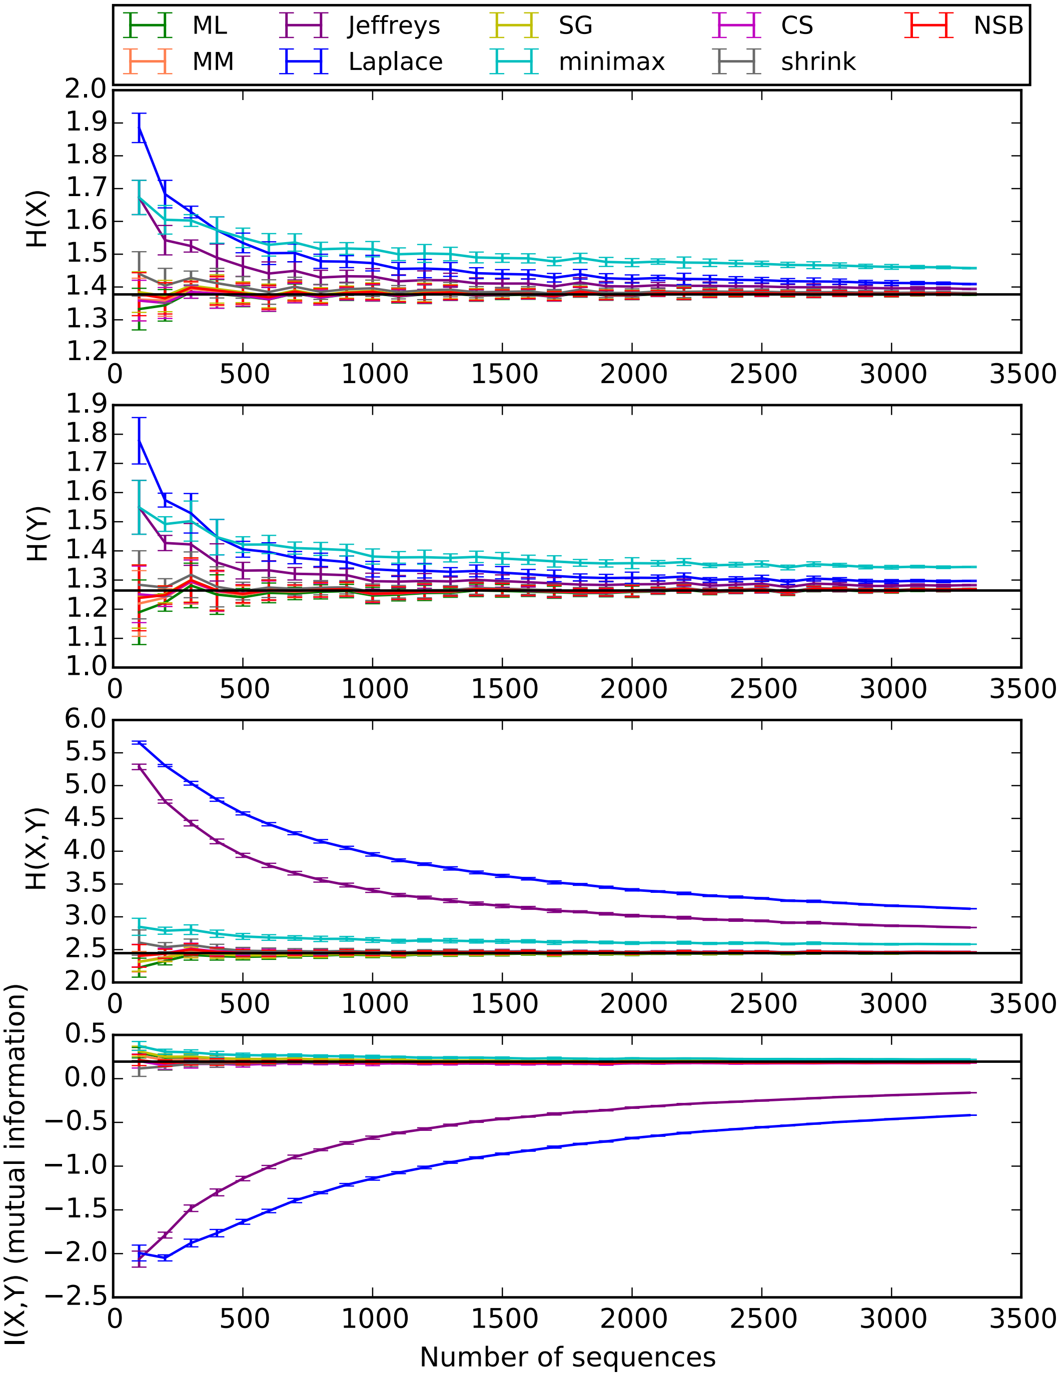


**Scaling of entropy and information estimators as a function of sample size.** Entropy for positions 54 ($X$) and 82 ($Y$) of HIV-1 protease as calculated by the different entropy estimators listed above, for increasing sample sizes (top two panels). The black horizontal lines represent empirical (maximum-likelihood) entropy estimates from all 3,399 sequences, and thus represent the "true" values that the estimators should achieve at smaller sample sizes. The lower two panels show the joint entropy and mutual information estimates for these two positions as a function of sample size. The NSB estimator appears to give the most reliable estimates of entropy and information down to samples as small as 100 sequences.

# References

[1] Bialek W. Biophysics: Searching for Principles. Princeton, N.J.: Princeton University Press; 2012.

[2] Miller G. Note on the bias of information estimates. Info Theory Psychol Prob Methods. 1955; II-B:95–100.

[3] Krichevsky RE, Trofimov VK. The performance of universal encoding. IEEE Trans Inf Theory. 1981; 27:199–207.

[4] Schurmann T, Grassberger P. Entropy estimation of symbol sequences. Chaos. 1996; 6:414–427.

[5] Chao A, Shen TJ. Nonparametric estimation of Shannon's index of diversity when there are unseen species in sample. Environ Ecol Stat. 2003; 10:429–443.

[6] Hausser J, Strimmer K. Entropy inference and the James-Stein estimator, with application to nonlinear gene association networks. J Mach Learn Res. 2009; 10:1469–1484.

[7] Nemenman I, Shafee F, Bialek W. Entropy and Inference, revisited. In: Adv Neural Inf Process Syst. vol. 14; 2002. p. 471–478.

[8] Wu TD, Schiffer CA, Gonzales MJ, Taylor J, Kantor R, Chou S, et al. Mutation patterns and structural correlates in human immunodeficiency virus type 1 protease following different protease inhibitor treatments. J Virol. 2003; 77:4836–4847.

# Supplementary Material: Strong Selection Pressure Significantly Increases Epistatic Interactions in the Long-Term Evolution of a Protein

A. Gupta and C. Adami

## Supplementary Text 7: Relationship between information and epistasis

To understand the relationship between residue co-variation and epistasis, we constructed a population genetic two-allele three-loci model. With 'A' and 'a' as the two alleles, the genotypes in the three-loci model are:
1: $AAA$
2: $AaA$
3: $aAA$
4: $Aaa$
5: $aAa$
6: $AAa$
7: $aaA$
8: $aaa$

If $\mu$ is the mutation rate per unit time, then the genotypes are generated from each other according to the figure below.

The probability to find each of these genotypes in an infinite population depends on the fitness and probabilities of the other genotypes. In a discrete update scheme, the probability to find type $i$ at time $t+1$ is related to the same quantity at time $t$ via

$$p_1^{t+1} = p_1^t \frac{w_1}{\bar{w}} F + \mu \left( \frac{p_2^t w_2 + p_3^t w_3 + p_6^t w_6}{\bar{w}} \right) + \mu^2 \left( \frac{p_4^t w_4 + p_5^t w_5 + p_7^t w_7}{\bar{w}} \right) + \mu^3 \frac{p_8^t w_8}{\bar{w}} \quad (1)$$

$$p_2^{t+1} = p_2^t \frac{w_2}{\bar{w}} F + \mu \left( \frac{p_1^t w_1 + p_4^t w_4 + p_7^t w_7}{\bar{w}} \right) + \mu^2 \left( \frac{p_3^t w_3 + p_6^t w_6 + p_8^t w_8}{\bar{w}} \right) + \mu^3 \frac{p_5^t w_5}{\bar{w}} \quad (2)$$

$$p_3^{t+1} = p_3^t \frac{w_3}{\bar{w}} F + \mu \left( \frac{p_1^t w_1 + p_5^t w_5 + p_7^t w_7}{\bar{w}} \right) + \mu^2 \left( \frac{p_2^t w_2 + p_6^t w_6 + p_8^t w_8}{\bar{w}} \right) + \mu^3 \frac{p_4^t w_4}{\bar{w}} \quad (3)$$

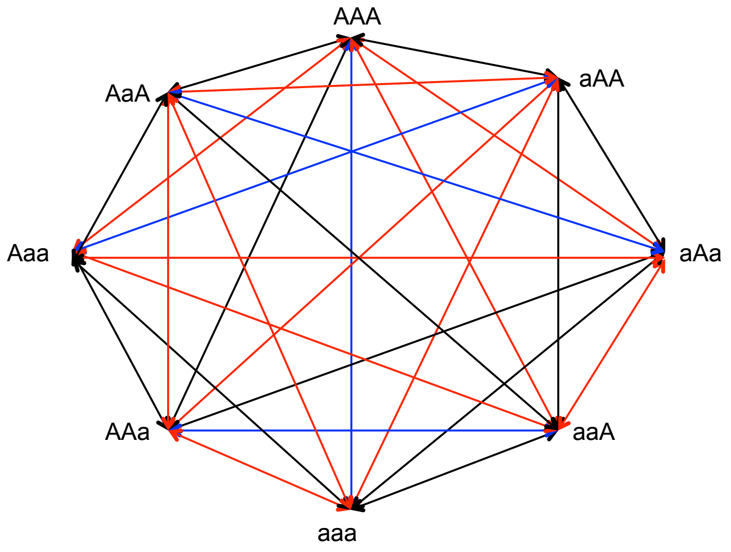


Rates of mutation between the eight different genotypes: black, red, and blue lines indicate that the connected genotypes are accessible by single, double, or triple mutations respectively (*i.e.* $\mu$, $\mu^2$, and $\mu^3$).

$$p_4^{t+1} = p_4^t \frac{w_4}{\bar{w}} F + \mu \left( \frac{p_2^t w_2 + p_6^t w_6 + p_8^t w_8}{\bar{w}} \right) + \mu^2 \left( \frac{p_1^t w_1 + p_5^t w_5 + p_7^t w_7}{\bar{w}} \right) + \mu^3 \frac{p_3^t w_3}{\bar{w}} \quad (4)$$

$$p_5^{t+1} = p_5^t \frac{w_5}{\bar{w}} F + \mu \left( \frac{p_3^t w_3 + p_6^t w_6 + p_8^t w_8}{\bar{w}} \right) + \mu^2 \left( \frac{p_1^t w_1 + p_4^t w_4 + p_7^t w_7}{\bar{w}} \right) + \mu^3 \frac{p_2^t w_2}{\bar{w}} \quad (5)$$

$$p_6^{t+1} = p_6^t \frac{w_6}{\bar{w}} F + \mu \left( \frac{p_1^t w_1 + p_4^t w_4 + p_5^t w_5}{\bar{w}} \right) + \mu^2 \left( \frac{p_2^t w_2 + p_3^t w_3 + p_8^t w_8}{\bar{w}} \right) + \mu^3 \frac{p_7^t w_7}{\bar{w}} \quad (6)$$

$$p_7^{t+1} = p_7^t \frac{w_7}{\bar{w}} F + \mu \left( \frac{p_2^t w_2 + p_3^t w_3 + p_8^t w_8}{\bar{w}} \right) + \mu^2 \left( \frac{p_1^t w_1 + p_4^t w_4 + p_5^t w_5}{\bar{w}} \right) + \mu^3 \frac{p_6^t w_6}{\bar{w}} \quad (7)$$

$$p_8^{t+1} = p_8^t \frac{w_8}{\bar{w}} F + \mu \left( \frac{p_4^t w_4 + p_5^t w_5 + p_7^t w_7}{\bar{w}} \right) + \mu^2 \left( \frac{p_2^t w_2 + p_3^t w_3 + p_6^t w_6}{\bar{w}} \right) + \mu^3 \frac{p_1^t w_1}{\bar{w}} \quad (8)$$

where $\bar{w}$ is the mean fitness $\bar{w} = \sum_{i=1}^{8} p_i^t w_i$, and $F$ is the fidelity of replication $F = 1 - 3\mu - 3\mu^2 - \mu^3$. It is easy to show that $\sum p_i^{t+1} = 1$ as long as $\sum p_i^t = 1$.

Equations (1-8) can be solved numerically iteratively, but alternatively the fixed point (the $p_i$ in the limit $t \to \infty$) can be calculated by solving for the right eigenvector of the associated Markov matrix.

Armed with the equilibrium probabilities $p_i$, we can calculate the information between loci as follows. First we define $p(A)$ and $p(a)$ for each of the three loci:

$$p^{(1)}(A) = p_1 + p_2 + p_4 + p_6 \ , \quad p^{(1)}(a) = 1 - p^{(1)}(A)$$

$$p^{(2)}(A) = p_1 + p_3 + p_5 + p_6 \ , \quad p^{(2)}(a) = 1 - p^{(2)}(A)$$
$$p^{(3)}(A) = p_1 + p_2 + p_3 + p_7 \ , \quad p^{(3)}(a) = 1 - p^{(3)}(A) \tag{9}$$

giving us the marginal entropies of the first and second locus

$$\begin{aligned} H(1) &= -\sum_{i=a,A} p^{(1)}(i) \log p^{(1)}(i) \ , \\ H(2) &= -\sum_{i=a,A} p^{(2)}(i) \log p^{(2)}(i) \ , \\ H(3) &= -\sum_{i=a,A} p^{(3)}(i) \log p^{(3)}(i) \ . \end{aligned} \tag{10}$$

The joint entropies for the pairwise loci are:

$$\begin{aligned} H(1,2) &= -\sum_{i=a,A} \sum_{j=a,A} p^{(1,2)}(i,j) \log p^{(1,2)}(i,j) \ , \\ H(1,3) &= -\sum_{i=a,A} \sum_{j=a,A} p^{(1,3)}(i,j) \log p^{(1,3)}(i,j) \ , \\ H(2,3) &= -\sum_{i=a,A} \sum_{j=a,A} p^{(2,3)}(i,j) \log p^{(2,3)}(i,j) \ . \end{aligned} \tag{11}$$

The shared entropies (or information) are

$$\begin{aligned} I(1:2) &= H(1) + H(2) - H(1,2) \ , \\ I(1:3) &= H(1) + H(3) - H(1,3) \ , \\ I(2:3) &= H(2) + H(3) - H(2,3) \ . \end{aligned} \tag{12}$$

Three-way epistasis in a two-allele three-loci model is defined as:

$$E = \log\left(\frac{w_{AAA} \times w_{aaa}}{w_{AaA} \times w_{aAA} \times w_{Aaa} \times w_{aAa} \times w_{AAa} \times w_{aaA}}\right)$$

The simulation is run for 4000 updates, with fitness landscape changing at the 2000th update as follows: starting with only the wild type genome as the most fit ($w_{AAA} = 1.0$), the fitness landscape becomes more rugged as the triple mutant become as fit as wild-type ($w_{AAA} = w_{aaa} = 1.0$). The fitnesses of the intermediate genotypes remain close to zero ($10^{-5}$) throughout the simulation.

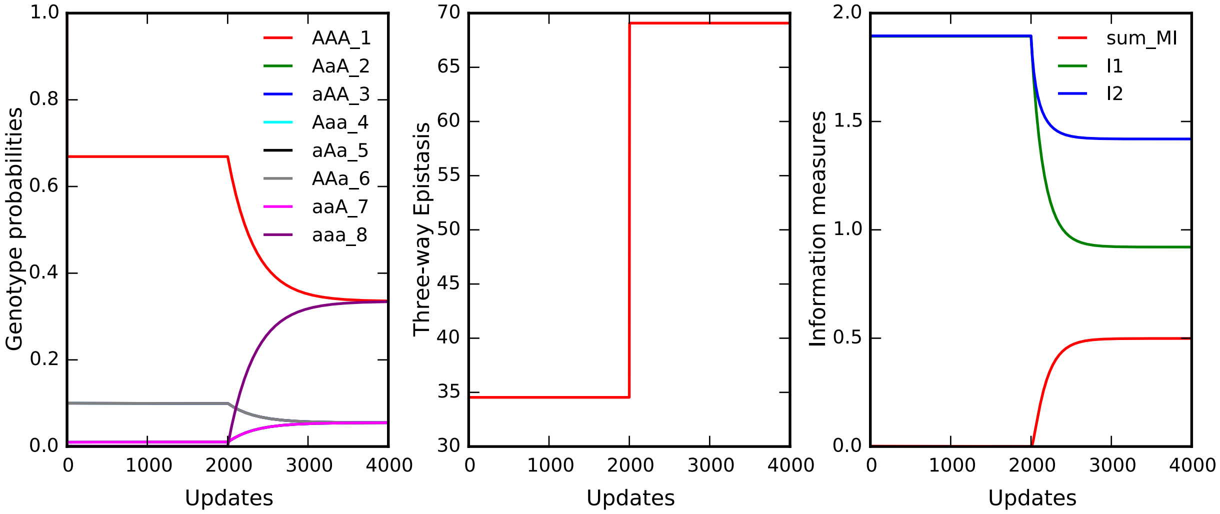


**Three-loci two-allele simulation.** Left panel shows the changes in genotype probabilities as the triple mutant ($aaa$) becomes as fit as the wild-type ($AAA$) at the 2000th update. Middle panel shows the increase in the three-way epistasis as the landscape becomes more rugged. Right panel shows the information measures: $I_1$, $I_2$, and sum of pairwise mutual information (MI). Notice that sum of MI increases with increase in epistasis.
